# Supplementary material for: Frustrated with Replicating Claims of a Shared Model? A Solution
Source: arXiv:1811.09737 source file (2019-06-25)
Supplement: Supplementary file 1 [file 99-supplementary.tex]

\section*{Supplementary Material}

\carml is a big system, and we had to selectively choose topics due to the space limitation.
This supplementary materials section is used to provide details about \carml that we were unable to cover in the paper's main body.

\subsection{Source Code}

This project is open-source and the code spans multiple ($>15$) repositories on GitHub.
Thus it is difficult to anonymize for the blind review process.
We are happy to share the links to the source code with the PC members. The links will be included in the paper after the blind review process.

\subsection{Model Manifests}

Listing~\ref{lst:ssd-mobilenet-coco} shows the manifest of \texttt{SSD\_MobileNet\_v1\_COCO}, an objection detection model, for TensorFlow.
This model embeds the pre-processing operations in the model graph, and thus requires no normalization, cropping, or resizing.
The major difference from a image classification model manifest is the task type (being \texttt{object\_detection}) and the outputs.
There are three output tensors for this model (boxes, probabilities, and classes).
These output tensors are processed by \carml to produce a single object detection feature array, which can then be visualized or used to calculate the metrics (e.g. mean average precision).
 
\begin{lstlisting}[
    language=yaml,
    escapeinside={(*}{*)},
    floatplacement=H,
    captionpos=b,
    label=lst:ssd-mobilenet-coco,
    caption={\carml's model specification for \texttt{SSD\_MobileNet\_v1\_COCO} TensorFlow model.
    },
    escapechar=|
]
name: SSD_MobileNet_v1_COCO  # name of your model
version: 1.0 # version information in semantic version format
task: object_detection # task type
framework:
  name: TensorFlow # framework name
  version: 1.12.x # framework version contraint
container: # containers used to perform model evaluation
  amd64:
    gpu: mlcn/tensorflow:amd64-cpu
    cpu: mlcn/tensorflow:amd64-gpu
  ppc64le:
    cpu: mlcn/tensorflow:ppc64le-gpu
    gpu: mlcn/tensorflow:ppc64le-gpu
description: ...
references: # references to papers / websites / etc.. describing the model
  - ...
license: Apache License, Version 2.0 # license of the model
inputs: # model inputs
  - type: image # first input modality
    element_type: uint8
    layer_name: image_tensor
    layout: HWC
    color_layout: RGB
outputs:
  - type: box
    element_type: float32
    layer_name: detection_boxes
  - type: probability
    element_type: float32
    layer_name: detection_scores
  - type: class
    element_type: float32
    layer_name: detection_classes
    features_url: https://.../labels.txt
source:
  graph_path: https://.../ssd_mobilenet_v1_coco_2018_01_28.pb
attributes: # extra model attributes
  training_dataset: COCO # dataset used to for training
  manifest_author: ...
\end{lstlisting}

Listing~\ref{lst:ssd-mask-rcnn-coco} shows the manifest of \texttt{Mask\_RCNN\_ResNet50\_v2\_Atrous\_COCO}, an instance segmentation model, for MXNet.
The major difference from the object detection model in Listing~\ref{lst:ssd-mobilenet-coco} is the task type (being \texttt{instance\_segmentation}) and the outputs.
Listing~\ref{lst:ssd-mask-rcnn-coco} shows four outputs for this model (boxes, probabilities, classes, and masks).
These output tensors are  processed by \carml to produce a single instance segmentation feature array.
Note that unlike TensorFlow, MXNet uses layer indices in place of layer names to get the tensor objects.

\begin{lstlisting}[
    language=yaml,
    escapeinside={(*}{*)},
    floatplacement=H,
    captionpos=b,
    label=lst:ssd-mask-rcnn-coco,
    caption={\carml's model specification for  \texttt{Mask\_RCNN\_ResNet50\_v2\_Atrous\_COCO} MXNet model.
    },
    escapechar=|
]
name: Mask_RCNN_ResNet50_v2_Atrous_COCO # name of your model
version: 1.0 # version information in semantic version format
task: instance_segmentation
framework:
  name: MXNet # framework for the model
  version: 1.4.x # framework version contraint
container: # containers used to perform model evaluation
  amd64:
    gpu: mlcn/mxnet:amd64-cpu
    cpu: mlcn/mxnet:amd64-gpu
  ppc64le:
    cpu: mlcn/mxnet:ppc64le-gpu
    gpu: mlcn/mxnet:ppc64le-gpu
description: ...
references: # references to papers / websites / etc.. describing the model
  - ...
license: Apache License, Version 2.0 # license of the model
inputs: # model inputs
  - type: image # first input modality
    element_type: uint8
    layout: HWC
    color_layout: RGB
outputs:
  - type: box
    element_type: float32
    layer_name: 0
  - type: probability
    element_type: float32
    layer_name: 1
  - type: class
    element_type: float32
    layer_name: 2
    features_url: https://.../labels.txt
  - type: mask
    element_type: float32
source: # specifies model graph and weights sources
  base_url: http://.../mxnet/Mask_RCNN_ResNet50_v2_Atrous_COCO/
  graph_path: model-symbol.json
  weights_path: model-0000.params
attributes: # extra model attributes
  training_dataset: COCO # dataset used to for training
  manifest_author: ...
\end{lstlisting}

\subsection{Website Workflow}

Although \carml provides both command line and library interfaces, we find the website provides an intuitive flow for specifying and running experiments.
Figure~\ref{fig:website_flow} shows the flow, and a video demonstrating it can be found at \url{https://drive.google.com/open?id=1LOXZ7hs_cy-i0-DVU-5FfHwdCd-1c53z}.
In figure~\ref{fig:website_flow}, users first arrive at  \circled{1} \carml's landing page.
The landing page contains a description of the project along with links to how to setup and install \carml.
Users can try \carml by \circled{2} clicking the demo button, which then displays \circled{3} the inference tasks exposed through the website.
If a user \circled{4} selects object detection, then \circled{5} models that are available for object detection are displayed.
A user can then \circled{7}  selects one or more models and \circled{8} selects one or more systems to run the evaluation on.
The input can be specified as a URL, data from disk, or dataset \circled{8} and once complete the user can perform the evaluation \circled{9}.
This \circled{10} will run the evaluation on the remote system and \circled{11} display the evaluation results along with summary of the execution flow.

\begin{figure}[h] 
    \centering
    \includegraphics[width=\textwidth]{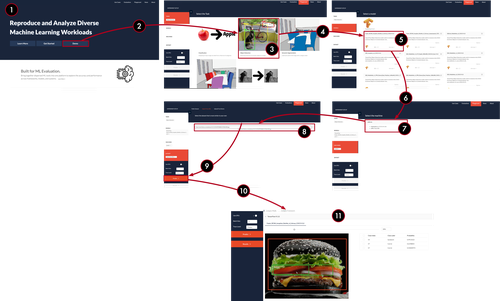}
    \caption{The \carml website provides an intuitive interface to conduct experiments.}
    \label{fig:website_flow}
    \vspace{-10pt}
\end{figure}
